# Supplementary material for: Exact hybrid particle/population simulation of rule-based models of biochemical systems
Source: arXiv:1301.6854 ancillary file (2014-02-05)
Supplement: Supplementary file 2 [file Dataset_S1_egfr_extended.pdf]

## egfr\_extended

egfr\_extended

population profiling

f=0.01

all species with mean pop >= 1 are reported

### Species

MEK(bind,loc~cyt,phos~U)  
ERK(bind!1,loc~cyt,phos~U).MEK(bind!1,loc~cyt,phos~U)  
ERK(bind,loc~cyt,phos~P)  
Ras(cat,nuc~GTP,raf)  
Ras(cat,nuc~GDP,raf)  
MEK(bind,loc~cyt,phos~P)  
PLCg(a,b~P,c~I)  
ERK(bind,loc~nuc,phos~U)  
ERK(bind,loc~nuc,phos~P)  
Shc(PTB,Y317~pY)  
ERK(bind,loc~cyt,phos~U)  
Egf(r)  
MEK(bind,loc~nuc,phos~U)  
ERK(bind!1,loc~nuc,phos~U).MEK(bind!1,loc~nuc,phos~U)  
Egfr(Y1068~Y,Y1148~Y,Y992~Y,d,I)  
Grb2(SH2!1,SH3).Shc(PTB,Y317~pY!1)  
Grb2(SH2!1,SH3!2).Shc(PTB,Y317~pY!1).Sos(dom!2,ras)  
ERK(bind!1,loc~cyt,phos~U).MEK(bind!1,loc~cyt,phos~P)  
Egf(r!1).Egfr(Y1068~Y,Y1148~Y,Y992~Y,d,!1)  
Grb2(SH2,SH3)  
Egf(r!1).Egf(r!2).Egfr(Y1068~Y,Y1148~Y,Y992~Y,d!3,!1).Egfr(Y1068~Y,Y1148~Y,Y992~Y,d!3,!2)  
MEK(bind,loc~nuc,phos~P)  
MEK(bind!1,loc~cyt,phos~U).Raf(bind!1,phos~P,ras!2).Ras(cat,nuc~GTP,raf!2)  
Shc(PTB,Y317~Y)  
Raf(bind,phos~P,ras!1).Ras(cat,nuc~GTP,raf!1)  
PLCg(a,b~P,c~0)  
ERK(bind!1,loc~nuc,phos~U).MEK(bind!1,loc~nuc,phos~P)  
Egf(r!1).Egf(r!2).Egfr(Y1068~Y,Y1148~Y,Y992~Y,d!3,!1).Egfr(Y1068~Y,Y1148~Y,Y992~pY,d!3,!2)  
Raf(bind,phos~U,ras)  
Egf(r!1).Egf(r!2).Egfr(Y1068~Y,Y1148~Y,Y992~Y,d!3,!1).Egfr(Y1068~pY,Y1148~Y,Y992~Y,d!3,!2)  
Egf(r!1).Egf(r!2).Egfr(Y1068~Y,Y1148~Y,Y992~Y,d!3,!1).Egfr(Y1068~Y,Y1148~pY,Y992~Y,d!3,!2)  
Grb2(SH2,SH3!1).Sos(dom!1,ras)  
Sos(dom,ras)  
PLCg(a,b~0,c~0)  
Egf(r!1).Egf(r!2).Egfr(Y1068~Y,Y1148~Y,Y992~Y,d!3,!1).Egfr(Y1068~Y,Y1148~pY!4,Y992~Y,d!3,!2).Shc(PTB!4,  
GAP(ras)  
Egf(r!1).Egf(r!2).Egfr(Y1068~Y,Y1148~Y,Y992~Y,d!3,!2).Egfr(Y1068~pY!4,Y1148~Y,Y992~Y,d!3,!1).Grb2(SH2!4  
GAP(ras!1).Ras(cat!1,nuc~GTP,raf)  
Egf(r!1).Egf(r!2).Egfr(Y1068~Y,Y1148~Y,Y992~Y,d!3,!1).Egfr(Y1068~pY!4,Y1148~Y,Y992~Y,d!3,!2).Grb2(SH2!4  
Egf(r!1).Egfr(Y1068~pY!2,Y1148~Y,Y992~Y,d,!1).Grb2(SH2!2,SH3)  
Egf(r!1).Egf(r!2).Egfr(Y1068~Y,Y1148~pY,Y992~Y,d!3,!1).Egfr(Y1068~pY,Y1148~Y,Y992~Y,d!3,!2)  
Egf(r!1).Egf(r!2).Egfr(Y1068~Y,Y1148~Y,Y992~pY,d!3,!2).Egfr(Y1068~pY,Y1148~pY,Y992~Y,d!3,!1)  
Egf(r!1).Egfr(Y1068~pY!2,Y1148~Y,Y992~Y,d,!1).Grb2(SH2!2,SH3!3).Ras(cat!4,nuc~GTP,raf).Sos(dom!3,ras!4)  
Egf(r!1).Egf(r!2).Egfr(Y1068~Y,Y1148~Y,Y992~Y,d!3,!1).Egfr(Y1068~pY,Y1148~Y,Y992~pY,d!3,!2)  
Egf(r!1).Egf(r!2).Egfr(Y1068~Y,Y1148~Y,Y992~pY,d!3,!2).Egfr(Y1068~pY,Y1148~Y,Y992~Y,d!3,!1)  
Egfr(Y1068~pY!1,Y1148~Y,Y992~Y,d,I).Grb2(SH2!1,SH3)  
Egf(r!1).Egf(r!2).Egfr(Y1068~Y,Y1148~Y,Y992~Y,d!3,!2).Egfr(Y1068~pY,Y1148~pY,Y992~Y,d!3,!1)

# egfr\_extended

Egf(r!1).Egf(r!2).Egfr(Y1068~Y,Y1148~Y,Y992~Y,d!3,!1).Egfr(Y1068~Y,Y1148~pY!4,Y992~Y,d!3,!2).Grb2(SH2!  
Egf(r!1).Egf(r!2).Egfr(Y1068~Y,Y1148~Y,Y992~Y,d!3,!2).Egfr(Y1068~Y,Y1148~pY,Y992~pY,d!3,!1)  
Egfr(Y1068~pY!1,Y1148~Y,Y992~Y,d,!).Grb2(SH2!1,SH3!2).Ras(cat!3,nuc~GTP,raf).Sos(dom!2,ras!3)  
Egf(r!1).Egfr(Y1068~Y,Y1148~pY!2,Y992~Y,d,!1).Shc(PTB!2,Y317~pY)  
Egf(r!1).Egf(r!2).Egfr(Y1068~Y,Y1148~Y,Y992~Y,d!3,!2).Egfr(Y1068~pY!4,Y1148~Y,Y992~Y,d!3,!1).Grb2(SH2!4

Mean Population

4094  
2333  
1386  
1213  
968  
665  
566  
498  
463  
450  
324  
316  
312  
307  
202  
202  
151  
106  
105  
86  
53  
50  
40  
27  
21  
17  
13  
11  
11  
11  
11  
11  
9  
9  
3  
3  
3  
2  
2  
2  
1  
1  
1  
1  
1  
1  
1

egfr\_extended

1  
1  
1  
1  
1
