# Supplementary material for: Exact hybrid particle/population simulation of rule-based models of biochemical systems
Source: arXiv:1301.6854 ancillary file (2014-02-05)
Supplement: Supplementary file 3 [file Dataset_S1_fceri_gamma2.pdf]

## fceri\_gamma2

fceri\_gamma2

population profiling

f=0.01

all species with mean pop >= 1 are reported

### Species

Lig(I,I)  
 Lyn(SH2,U)  
 Rec(a,b~Y,g~Y,g~Y)  
 Lig(I!1,I!2).Lyn(SH2!3,U).Lyn(SH2!4,U).Rec(a!1,b~pY!3,g~Y,g~Y).Rec(a!2,b~pY!4,g~Y,g~Y)  
 Lig(I!1,I!2).Lyn(SH2!3,U).Lyn(SH2!4,U).Rec(a!1,b~pY!3,g~Y,g~Y).Rec(a!2,b~pY!4,g~Y,g~pY)  
 Lyn(SH2,U!1).Rec(a,b~Y!1,g~Y,g~Y)  
 Lig(I!1,I!2).Lyn(SH2!3,U).Lyn(SH2!4,U).Rec(a!1,b~pY!3,g~Y,g~Y).Rec(a!2,b~pY!4,g~Y,g~pY!5).Syk(a~Y,l~pY,tSH2)  
 Lig(I!1,I!2).Lyn(SH2!3,U).Rec(a!1,b~pY!3,g~Y,g~Y).Rec(a!2,b~pY,g~Y,g~Y)  
 Lig(I!1,I!2).Lyn(SH2!3,U).Lyn(SH2!4,U).Rec(a!1,b~pY!3,g~Y,g~pY).Rec(a!2,b~pY!4,g~Y,g~pY)  
 Lig(I!1,I!2).Lyn(SH2!3,U).Lyn(SH2!4,U).Rec(a!1,b~pY!3,g~Y,g~pY!5).Rec(a!2,b~pY!4,g~Y,g~pY).Syk(a~Y,l~pY,tSH2)  
 Lig(I!1,I!2).Lyn(SH2!3,U).Lyn(SH2!4,U).Rec(a!1,b~pY!3,g~Y,g~Y).Rec(a!2,b~pY!4,g~pY,g~pY)  
 Lig(I!1,I!2).Lyn(SH2!3,U).Lyn(SH2!4,U).Rec(a!2,b~pY!4,g~Y,g~Y).Rec(a!1,b~pY!3,g~Y,g~pY!5).Syk(a~Y,l~Y,tSH2)  
 Lig(I!1,I!2).Lyn(SH2!3,U).Rec(a!1,b~pY!3,g~Y,g~Y).Rec(a!2,b~pY,g~Y,g~pY)  
 Lig(I!1,I!2).Rec(a!1,b~Y,g~Y,g~Y).Rec(a!2,b~Y,g~Y,g~Y)  
 Lig(I!1,I!2).Lyn(SH2!3,U).Lyn(SH2!4,U).Rec(a!1,b~pY!3,g~Y,g~Y).Rec(a!2,b~pY!4,g~pY!5,g~pY).Syk(a~Y,l~pY,tSH2)  
 Syk(a~Y,l~Y,tSH2)  
 Lig(I!1,I!2).Lyn(SH2!3,U).Rec(a!1,b~Y,g~Y,g~Y).Rec(a!2,b~pY!3,g~Y,g~Y)  
 Lig(I!1,I!2).Lyn(SH2!3,U).Lyn(SH2!4,U).Rec(a!1,b~pY!3,g~Y,g~pY).Rec(a!2,b~pY!4,g~pY,g~pY)  
 Lig(I!1,I!2).Lyn(SH2!3,U).Lyn(SH2!4,U).Rec(a!2,b~pY!4,g~Y,g~pY!5).Rec(a!1,b~pY!3,g~Y,g~pY).Syk(a~Y,l~Y,tSH2)  
 Lig(I!1,I!2).Lyn(SH2!3,U).Lyn(SH2!4,U).Rec(a!1,b~pY!3,g~Y,g~pY!5).Rec(a!2,b~pY!4,g~Y,g~pY!6).Syk(a~pY,l~pY)  
 Lig(I!1,I!2).Lyn(SH2!3,U).Rec(a!1,b~pY!3,g~Y,g~Y).Rec(a!2,b~pY,g~Y,g~pY!4).Syk(a~Y,l~pY,tSH2!4)  
 Lig(I!1,I!2).Lyn(SH2!3,U).Lyn(SH2!4,U).Rec(a!2,b~pY!4,g~Y,g~pY).Rec(a!1,b~pY!3,g~pY!5,g~pY).Syk(a~Y,l~pY,tSH2!4)  
 Lig(I!1,I!2).Lyn(SH2!3,U).Rec(a!1,b~pY!3,g~Y,g~pY!4).Rec(a!2,b~pY,g~Y,g~Y).Syk(a~Y,l~Y,tSH2!4)  
 Lig(I!1,I!2).Lyn(SH2!3,U).Rec(a!2,b~Y,g~Y,g~pY).Rec(a!1,b~pY!3,g~Y,g~Y)  
 Lig(I!1,I!2).Lyn(SH2!3,U).Lyn(SH2!4,U).Rec(a!1,b~pY!3,g~Y,g~Y).Rec(a!2,b~pY!4,g~pY!5,g~pY).Syk(a~Y,l~Y,tSH2!4)  
 Lig(I!1,I!2).Lyn(SH2!3,U).Lyn(SH2!4,U).Rec(a!1,b~pY!3,g~Y,g~Y).Rec(a!2,b~pY!4,g~pY!5,g~pY!6).Syk(a~Y,l~pY,tSH2!4)  
 Lig(I!1,I!2).Lyn(SH2,U!3).Rec(a!1,b~Y!3,g~Y,g~Y).Rec(a!2,b~Y,g~Y,g~Y)  
 Lig(I!1,I!2).Lyn(SH2!3,U).Lyn(SH2!4,U).Rec(a!1,b~pY!3,g~Y,g~pY!5).Rec(a!2,b~pY!4,g~pY,g~pY).Syk(a~Y,l~pY,tSH2!4)  
 Lig(I!1,I!2).Lyn(SH2!3,U).Lyn(SH2!4,U).Rec(a!1,b~pY!3,g~Y,g~pY!5).Rec(a!2,b~pY!4,g~Y,g~pY!6).Syk(a~pY,l~Y,tSH2!4)  
 Lig(I!1,I!2).Lyn(SH2,U!3).Rec(a!2,b~Y!3,g~Y,g~Y).Rec(a!1,b~pY,g~Y,g~Y)  
 Lig(I!1,I!2).Lyn(SH2!3,U).Lyn(SH2,U!4).Rec(a!1,b~Y!4,g~Y,g~Y).Rec(a!2,b~pY!3,g~Y,g~Y)  
 Lig(I!1,I!2).Rec(a!1,b~Y,g~Y,g~Y).Rec(a!2,b~Y,g~Y,g~pY!3).Syk(a~Y,l~Y,tSH2!3)  
 Lig(I!1,I!2).Rec(a!1,b~Y,g~Y,g~Y).Rec(a!2,b~pY,g~Y,g~Y)  
 Lig(I!1,I!2).Lyn(SH2!3,U).Rec(a!1,b~pY!3,g~Y,g~pY).Rec(a!2,b~pY,g~Y,g~Y)  
 Lig(I!1,I!2).Lyn(SH2!3,U).Lyn(SH2!4,U).Rec(a!2,b~pY!4,g~Y,g~pY!5).Rec(a!1,b~pY!3,g~pY!6,g~pY).Syk(a~pY,l~Y,tSH2!4)  
 Lig(I!1,I!2).Lyn(SH2!3,U).Rec(a!2,b~pY!3,g~Y,g~Y).Rec(a!1,b~pY,g~pY,g~pY)  
 Lig(I!1,I!2).Lyn(SH2!3,U).Rec(a!1,b~pY!3,g~Y,g~pY!4).Rec(a!2,b~pY,g~Y,g~pY).Syk(a~Y,l~Y,tSH2!4)  
 Lig(I!1,I!2).Lyn(SH2!3,U).Rec(a!1,b~pY!3,g~Y,g~Y).Rec(a!2,b~pY!4,g~pY!5,g~pY!6).Syk(a~Y,l~Y,tSH2!4)  
 Lig(I!1,I!2).Lyn(SH2!3,U).Rec(a!2,b~Y,g~Y,g~pY!4).Rec(a!1,b~pY!3,g~Y,g~Y).Syk(a~Y,l~pY,tSH2!4)  
 Lig(I!1,I!2).Lyn(SH2!3,U).Lyn(SH2!4,U).Rec(a!2,b~pY!4,g~Y,g~pY).Rec(a!1,b~pY!3,g~pY!5,g~pY).Syk(a~Y,l~Y,tSH2)  
 Syk(a~Y,l~pY,tSH2)  
 Lig(I!1,I!2).Lyn(SH2!3,U).Lyn(SH2!4,U).Rec(a!1,b~pY!3,g~Y,g~pY!5).Rec(a!2,b~pY!4,g~Y,g~pY!6).Syk(a~Y,l~pY,tSH2!4)

Mean Population

58745  
959  
788  
623  
372  
261  
119  
61  
56  
36  
27  
24  
18  
18  
18  
15  
12  
8  
6  
5  
5  
5  
5  
4  
4  
3  
3  
3  
2  
2  
2  
2  
2  
2  
2  
1  
1  
1  
1  
1  
1  
1  
1
