# Supplementary material for: Exact hybrid particle/population simulation of rule-based models of biochemical systems
Source: arXiv:1301.6854 ancillary file (2014-02-05)
Supplement: Supplementary file 4 [file Dataset_S1_tlbr.pdf]

tlbr

tlbr

population profiling

f=0.01

all species with mean pop >= 1 are reported

# Species

L(r,r,r)  
R(l,l)  
L(r,r,r!1).R(l,!1)  
L(r,r,r!1).L(r,r,r!2).R(!2,!1)  
L(r,r,r!1).L(r,r,r!2).L(r,r!3,r!4).R(!2,!3).R(!1,!4)  
L(r,r,r!1).L(r,r,r!2).R(!2,!1).R(l,!3)  
L(r,r,r!1).L(r,r,r!2).L(r,r!3,r!4).L(r,r!5,r!6).R(!4,!6).R(!3,!2).R(!5,!1)  
L(r,r!1,r!2).R(l,!2).R(l,!1)  
L(r,r!1,r!2).L(r,r!3,r!4).L(r,r,r!5).R(!1,!3).R(!2,!5).R(l,!4)  
L(r,r!1,r!2).L(r,r!3,r!4).L(r,r!5,r!6).L(r,r,r!7).L(r,r,r!8).R(!5,!1).R(!3,!2).R(!6,!7).R(!4,!8)  
L(r,r!1,r!2).L(r,r!3,r!4).L(r,r!5,r!6).L(r,r,r!7).R(!1,!3).R(!2,!5).R(!4,!7).R(l,!6)  
L(r!1,r!2,r!3).R(l,!3).R(l,!2).R(l,!1)  
L(r,r!1,r!2).L(r,r!3,r!4).R(!4,!2).R(l,!3).R(l,!1)  
L(r!1,r!2,r!3).L(r,r,r!4).L(r,r,r!5).R(!1,!5).R(!2,!4).R(l,!3)  
L(r,r!1,r!2).L(r,r!3,r!4).L(r,r!5,r!6).L(r,r!7,r!8).L(r,r,r!9).L(r,r,r!10).R(!4,!2).R(!3,!5).R(!1,!7).R(!6,!9).R(!8,!10)  
L(r!1,r!2,r!3).L(r,r!4,r!5).L(r,r,r!6).L(r,r,r!7).L(r,r,r!8).R(!8,!5).R(!7,!1).R(!6,!2).R(!4,!3)  
L(r!1,r!2,r!3).L(r,r!4,r!5).L(r,r,r!6).L(r,r,r!7).R(!7,!5).R(!6,!1).R(!4,!2).R(l,!3)  
L(r!1,r!2,r!3).L(r,r,r!4).R(!3,!4).R(l,!2).R(l,!1)  
L(r!1,r!2,r!3).L(r,r!4,r!5).R(!3,!5).R(l,!2).R(l,!1).R(l,!4)  
L(r,r,r!1).L(r,r,r!2).L(r,r,r!3).L(r!4,r!5,r!6).R(!3,!4).R(!2,!5).R(!1,!6)  
L(r,r!1,r!2).L(r,r!3,r!4).L(r,r!5,r!6).L(r,r!7,r!8).L(r,r,r!9).R(!1,!3).R(!2,!5).R(!4,!7).R(!6,!9).R(l,!8)  
L(r!1,r!2,r!3).L(r,r!4,r!5).L(r,r,r!6).R(!1,!6).R(!2,!4).R(l,!3).R(l,!5)  
L(r!1,r!2,r!3).L(r,r!4,r!5).L(r,r!6,r!7).L(r,r,r!8).L(r,r,r!9).L(r,r,r!10).R(!7,!8).R(!5,!9).R(!6,!1).R(!4,!2).R(!10,!3)  
L(r!1,r!2,r!3).L(r,r!4,r!5).L(r,r,r!6).L(r,r,r!7).R(!4,!3).R(!7,!1).R(!6,!2).R(l,!5)

tlbr

Mean Population

47222

74

44

43

21

17

9

9

7

4

4

3

2

2

2

2

2

2

2

2

1

1

1

1
